# Supplementary material for: Joint Learning of Portrait Intrinsic Decomposition and Relighting
Source: arXiv:2106.15305 source file (2021-06-22)
Supplement: Supplementary file 1 [file supp.tex]

\documentclass[10pt,twocolumn,letterpaper]{article}

\usepackage{cvpr}
\usepackage{times}
\usepackage{epsfig}
\usepackage{graphicx}
\usepackage{amsmath}
\usepackage{amssymb}
\usepackage{subcaption}
\usepackage{multirow}
\usepackage{graphics}
\usepackage{pifont}
\usepackage{float}

% Include other packages here, before hyperref.

% If you comment hyperref and then uncomment it, you should delete
% egpaper.aux before re-running latex.  (Or just hit 'q' on the first latex
% run, let it finish, and you should be clear).
\usepackage[pagebackref=true,breaklinks=true,letterpaper=true,colorlinks,bookmarks=false]{hyperref}

% \cvprfinalcopy % *** Uncomment this line for the final submission

 % *** Enter the CVPR Paper ID here

% Pages are numbered in submission mode, and unnumbered in camera-ready
\ifcvprfinal\pagestyle{empty}\fi

% \date{\includegraphics[height=2in]{draft/figures/light_transfer/pics.png}}

\begin{document}

% commands
\newcommand{\mz}[1]{\textsf{\textbf{\color{blue}{\tiny [MZ: #1]}}}}
\newcommand{\sg}[1]{\textsf{\textbf{\color{magenta}{\tiny [SG: #1]}}}}
\newcommand{\cmark}{\ding{51}}%
\newcommand{\xmark}{\ding{55}}%

%%%%%%%%% TITLE
\title{Joint Learning of Shape from Image and Portrait Relighting \\ Supplementary Material}
% \title{Joint Learning of Portrait Intrinsic Decomposition and Relighting}

\author{First Author\\
Institution1\\
Institution1 address\\
{\tt\small firstauthor@i1.org}
% For a paper whose authors are all at the same institution,
% omit the following lines up until the closing ``}''.
% Additional authors and addresses can be added with ``\and'',
% just like the second author.
% To save space, use either the email address or home page, not both
\and
Second Author\\
Institution2\\
First line of institution2 address\\
{\tt\small secondauthor@i2.org}
}

\maketitle

%\thispagestyle{empty}
% \begin{center} 
% \centering
% \includegraphics[width=1\linewidth]{draft/figures/light_transfer/pics.png}
% \captionof{figure}{Quality of decomposition and relighting in experiments trained only on Multi-lit CelebA dataset with light supervision, with and without cross-relighting loss term.}
% \label{fig:pics}
% \end{center}

% \newpage
\input{sections/appendix.tex}

{\small
\bibliographystyle{ieee_fullname}
\bibliography{sections/refs.bib}
}

\end{document}
